# Supplementary material for: The Cost of Representation by Subset Repairs
Source: arXiv:2410.16501 source file (2024-10-21)
Supplement: Supplementary file 1 [file appendix_lhsmarriage_RP.tex]

\section{A Randomized Polynomial-time (RP) Algorithm for Optimal \rsrepair{} for Simple LHS Marriage}\label{sec:rp-algo-simple-lhs-marriage}
The following theore shows that LHS marriage has a randomized poly-time algorithm like the exact colored matching problem (hence it is not NP-hard unless {\tt NP = RP}). It remains open to study the general class of \rsrepair{}s that entails a randomized polynomial time algorithm.
\begin{theorem}
The following results hold:
    \begin{itemize}
        %\item \blue{There is a polynomial-time reduction from the exact colored matching problem to the decision problem of finding an optimal \rsrepair{} for simple LHS marriage  (see \Cref{lem:ecm_to_simple_lhs})}
        \item There is a polynomial-time reduction from the problem of finding an \rsrepair{} for simple LHS marriage to the exact colored matching problem (see \Cref{lem:simple_lhs_reduce})
        \item The exact colored matching problem \cut{simple LHS marriage for representative repair}has a randomized polynomial-time algorithm (see \Cref{lem:randomized})
    \end{itemize}
\end{theorem}

\begin{lemma}\label{lem:simple_lhs_reduce}
    The problem of finding an \rsrepair{} for simple LHS marriage can be reduced to an exact colored matching problem in polynomial time.
    %, where $\phi_i$ is the number of edges in color $i$ in a matching $M$.
     %$\rc{} = (\phi_1, \phi_2, \cdots, \phi_k)$ 
\end{lemma}
\begin{proof}
    Given an instance of finding an \rsrepair{} for simple LHS marriage\cut{\prob{ (\relation{},\fdset{},\rc{})}}, we construct an instance of the exact colored matching problem as follows:
    \begin{itemize}
        \item Construct an unweighted bipartite graph $G = (U \cup V, E)$, where $U$ and $V$ are disjoint node sets based on the distinct values of attributes $A$ and $B$ in $\relation{}$, respectively. Formally, $U = \{u \mid \exists t \in \relation{} \text{ s.t. } t[A] = u\}$ and $V = \{v \mid \exists t \in \relation{} \text{ s.t. } t[B] = v\}$. The edge set $E$ connects nodes from $U$ to nodes from $V$, i.e., $E = \{(u, v) \mid \exists t \in \relation{} \text{ s.t. } t[A] = u \text{ and } t[B] = v\}$.
        \item Each edge $(u, v) \in E$ is assigned a color corresponding to the value of the sensitive attribute $C$ in the tuple $t \in \relation{}$ where $t[A] = u$ and $t[B] = v$.
        \item Define the color constraint $\phi = (\phi_1, \phi_2, \cdots, \phi_k)$, where $\phi_i = |E| \cdot \rc_i$ is the number of edges in color $i$ that should be present in the matching $M$.
    \end{itemize}
    %1) construct a bipartite graph $G=(U \cup V,E)$ that consists two disjoint nodes sets $U$ and $V$ based on the distinct values of $X$ and $Y$ in $R$ \yuxi{based on $\pi_{X}{\relation{}}$ and $\pi_{Y}{\relation{}}$?}, i.e., $U = \{u \mid \exists t \in R \text{ such that } t[X] = u\}$ and $V = \{v \mid \exists t \in R \text{ such that } t[Y] = v\}$. An edge set $E$ connecting nodes from $U$ to nodes from $V$, i.e., $E = \{(u, v) \mid \exists t \in R \text{ s.t. } t[X] = u \text{ and } t[Y] = v\}$. 2) each edge $(u,v)$ is assigned to a color corresponding to the value of the sensitive attribute $A_{\ell}$ in the tuple $t \in \relation$ where $t[X] = u$ and $t[Y] = v$; 3) define the color constraint $\rc' = (\rc_1, \rc_2, \cdots, \rc_k)$, where $\rc_{i}$ is the number of edges in color $i$ that should be satisfied in the matching $M$.

    We prove that there\cut{\prob{ (\relation{},\fdset{},\rc{})}} exists an \rsrepair{} $\relation'$ if and only if there is an exact colored matching $M$ in $G$ satisfying $\phi$. 
    
    \paragraph*{($\Rightarrow$)} Suppose $G$ has a matching $M$ that satisfies $\phi$. We construct an \rsrepair{} $\relation{}'$ as follows: for each edge $(u, v)$ in $M$, add the corresponding tuple $t$ to $\relation{}'$ where $t[A] = u$, $t[B] = v$, and $t[C]$ is the color of the edge $(u, v)$. Since $M$ is a valid matching in $G$, for any two edges $(u_1, v_1)$ and $(u_2, v_2)$ in $M$, we have $u_1 \neq u_2$ and $v_1 \neq v_2$. This implies that for any two tuples $t_1, t_2 \in \relation{}'$, $t_1[A] \neq t_2[A]$ and $t_1[B] \neq t_2[B]$. So $\relation{}'$ satisfies the FDs in $\fdset{}$. Furthermore, since $M$ satisfies the color constraint $\phi$, the number of tuples with each sensitive attribute value $c_i$ in $\relation{}'$ is equal to $\phi_i = |E| \cdot \rc_i$. Thus, $\relation{}'$ satisfies the RC $\rc{}$. Therefore, $\relation{}'$ is an \rsrepair{}.

    \paragraph*{($\Leftarrow$)} Suppose there is an \rsrepair{} $\relation{}'$. We construct an exact colored matching $M$ in $G$ as follows: for each tuple $t$ in $\relation{}'$, add the corresponding edge $(t[A], t[B])$ to $M$. Since $\relation{}'$ satisfies the FDs in $\fdset{}$, for any two tuples $t_1, t_2 \in \relation{}'$, if $t_1[A] = t_2[A]$, then $t_1[B] = t_2[B]$. This implies that $M$ is a valid matching in $G$. Furthermore, since $\relation{}'$ satisfies the RC $\rc{}$, the number of edges in color $i$ in $M$ is equal to $|\relation{}'| \cdot \rc_i$. By the construction of $G$, we have $|\relation{}'| = |M| = |E|$. Thus, the number of edges in color $i$ in $M$ is equal to $|E| \cdot \rc_i = \phi_i$, satisfying the color constraint $\phi$.

    The reduction can be done in polynomial time as it scans the tuples in $\relation{}$ once to construct the graph $G$ and sets the color constraint $\phi$ based on $|E|$ and $\rc{}$.

\end{proof}

\red{Why Lemma 20 does not give an RP algo for Optimal RS repair?}

We present \Cref{alg:randomized} for finding an \red{optimal} \rsrepair{} for LHS marriage. \red{This algorithm is adapted from the ideas presented for color-balanced bipartite matching from ???, which }. % for \Cref{lem:randomized}.
%Then we show that the exact colored matching problem can also be reduced to the simple LHS Marriage in polynomial time.
\begin{lemma}\label{lem:randomized}
        The exact colored matching problem can be solved by a randomized polynomial time algorithm. The algorithm will output a matching $M$ satisfying $\phi = (\phi_1, \phi_2, \cdots, \phi_k)$ with a probability of at least $\frac{1}{2}$ if such matching exists and will produce NO with a probability of 1 if there is no matching satisfying $\phi$ in $G$.
        %Given an unweighted bipartite graph $G=(U\cup V, E)$ with each edge colored either red or blue, and a color constraint $\phi = (\phi_1, \phi_2)$, the problem of finding a maximum matching $M$ with $\phi_1$ red edges and $\phi_2$ blue edges\cut{i.e. the edge color distribution satisfies $\sigma(M)=\phi$.} can be solved by a randomized polynomial time algorithm. 

        %The algorithm will output a maximum matching $M$ with $\phi_1$ red edges and $\phi_2$ blue edges with a probability at least $\frac{1}{2}$ if such matching exists and will produce NO with a probability 1 if there is no matching satisfying $\phi_1$ red edges and $\phi_2$ blue edges in $G$.
\end{lemma}

\cut{
Our algorithm extends the ideas from Mulmuley et al.~\cite{mulmuley1987matching} and Santhini et al.~\cite{ka2022optimal-AAMAS22}. Here we give a proof sketch. %The algorithm and the full proof are in the appendix.

\underline{Proof Sketch.}
The algorithm starts by extending the input bipartite graph $G$ to a complete bipartite graph $G^*$. Let $G^* = (U^*, V^*, E^*)$ be a complete bipartite graph extended from a bipartite graph $G=(U,V,E)$ by adding dummy vertices and new edges. Old edges from $G$ remain in their colors, and new edges are not colored. Then we assign the random weights according to the process from ~\cite{mulmuley1987matching} as follows: assign weights to each edge $e \in E^*$ uniformly and randomly from $[1, 2m]$ and then add $2mn$ to the weight of each new edge added, where $n = |U^*| = |V^*|$ and $m = |E^*| = n^2$. As a result, finding the Exact Colored Matching is reduced to finding a minimum weight perfect matching with same color constraint \rc{} in $G^*$ (Lemma \ref{lem:max_to_perfect}). Denote the perfect matching satisfying \rc{} in $G^*$ as \textit{Exact Matching with Constraint (EMC)}. Next, we prove how to find the minimum weight EMC in $G^*$.

We use the modified isolation lemma to ensure the $G^*$ has a unique minimum weight EMC with probability at least $\frac{1}{2}$ (Lemma \ref{lem:isolation}). %The proof is identical to ~\cite{mulmuley1987matching}. 
Then we construct a modified adjacency matrix $B$:
\begin{equation*}
B_{u,v} = \begin{cases}
    0 & \text{if } (u,v) \notin E^* \\
    2^{w_e}y_i & \text{if } (u,v) \in E^* \text{ with color } i \\
    2^{w_e} & \text{if } (u,v) \in E^* \text{ with no color}
\end{cases}
\end{equation*}  
where $y_1, \cdots, y_k$ are new variables defined to represent the edges' color in the matrix. $w_e$ is the random weight we assign to each edge $e \in E^*$.

If there exists an EMC in $G^*$, then the coefficient of $\prod_{i=1}^k{y_i}^{\phi_i}$ in $det(B)$
\benny{Please avoid writing words in math. Latex thinks that this is a multiplication of three factors. Use $\mathrm{det}$ or $\mbox{det}$.}
is non-zero with probability $\geq \frac{1}{2}$ (Lemma \ref{lemma: non_zero_coef}). % We also prove a modified version of the Isolation Lemma to ensure a unique minimum weight matching satisfying the color constraint with high probability (Lemma 3).
Finally, we use the coefficients of $\prod_{i=1}^k{y_i}^{\phi_i}$ in $det(B)$ and the adjoint matrix of B to identify the edges belonging to the minimum weighted EMC (Lemma \ref{lem: find_edge}).

The time complexity of the algorithm is at most $O(n^{k^2+4})$, which is polynomial when $k$ is constant.  The full proof is provided in the appendix.
}

 First, we show the correctness of \Cref{lem:randomized}, and then 
%is proved in \Cref{subsec:appendix_random_proof} and 
give the time complexity analysis is in \Cref{subsec:randomized_time}.
\begin{algorithm}
    \caption{Randomized Algorithm for Exact Colored Matching}\label{alg:randomized}
    \begin{algorithmic}[1]
    \Require{Unweighted bipartite graph $G=(U,V,E)$ with each $e \in E$ colored by one of $k$ colors; constraint $\phi = (\phi_1, \phi_2, \cdots, \phi_k)$}
    \Ensure{An exact colored matching $M$ or "No matching satisfies $\phi$" }
    \State Extend $G$ to a complete bipartite graph $G^*=(U^*, V^*, E^*)$ by adding dummy vertices and uncolored new edges.
    % \State Assign random weights to each edge $e \in E^$:
    % \begin{itemize}
    % \item If $e$ is an original edge from $E$, assign a weight uniformly and randomly from $[1, 2m]$.
    % \item If $e$ is a new edge, assign a weight uniformly and randomly from $[1, 2m]$ and add $2mn$ to it.
    % \end{itemize}
    % \Comment{$m=|E^*|$ and $n = |V^*|$}
    \State Assign weight to each edge $e \in E^*$ uniformly and randomly chosen from $[1, 2m]$. Then add $2mn$ to the weight of each new edge added. \Comment{$m=|E^*|$ and $n = |V^*|$}
    \State Construct the adjacency matrix $B$ for $G^*$.
    $$B_{u,v}=
    \begin{cases}
    0 & \text{if } (u,v) \notin E^* \\
    2^{w_e}y_i & \text{if } (u,v) \in E^* \text{ with color } i \\
    2^{w_e} & \text{if } (u,v) \in E^* \text{ is uncolored}
    \end{cases}
    $$
    \Comment{$y_1,y_2,\cdots, y_k$ are new variables representing edge colors}
    \State Obtain $det(B)$ \Comment{$det(B)$ is a polynomial in $y_1,y_2, \cdots, y_k$}
    \State Compute the coefficient $\alpha$ of $\prod_{i=1}^k{y_i}^{\phi_i}$ in $det(B)$. 
    \State Check $\alpha$; if $\alpha = 0$ then return "No matching satisfies $\phi$"
    \State Obtain $w$ such that $2^w$ is the highest power of 2 dividing $\alpha$
    \State Compute the adjoint matrix $adj(B)$ \Comment{The $(i,j)^{th}$ entry of $adj(B)$ is $det(B_{ij})$}
    \State For each edge $(u_i, v_j) \in E^*$ do in parallel:
        \begin{itemize}
            \item Compute $\frac{\alpha_{ij}}{2^w}$ \Comment{$\alpha_{ij}$ is the coefficient of $\prod_{i=1}^k{y_i}^{\phi_i}$ for $det(B_{ij})b_{ij}$}
            \item If $\frac{\alpha_{ij}}{2^w}$ is odd, include $(u_i, v_j)$ in the matching $M^*$
        \end{itemize}
    \State Check whether $M^*$ is a perfect matching in $G^*$ satisfying $\phi$: %Check whether the selected edges form a perfect matching $M^*$ satisfying \rc{} in $G^*$:
        \begin{itemize}
            \item If yes, remove vertices and edges added at Line 1 and output the corresponding matching $M$ in $G$;
            \item if no\cut{(the probability of this case is at most $\frac{1}{2}$)}, repeat from Line 2.
        \end{itemize}

\end{algorithmic}
\end{algorithm}

%\subsection{Algorithm of Simple LHS Marriage}\label{sec:appendix_random_algo}

%\subsection{Proof of Lemma~\ref{lem:randomized}}\label{subsec:appendix_random_proof}
We proved the correctness in four steps:
\subsubsection{Reduction to Minimum Weight Perfect Matching}
~We reduce the problem of finding an exact colored matching in $G$ to finding a minimum weight perfect matching satisfying the color constraint $\phi$ in the complete bipartite graph $G^*$, constructed as follows \cite{mulmuley1987matching}:
\begin{itemize}
\item Extend $G$ to a complete bipartite graph $G^*=(U^*, V^*, E^*)$ by adding dummy vertices and edges. Old edges from $G$ remain in their colors, and new edges are not colored.
\item Assign weights to each edge $e \in E^*$ randomly from $[1, 2m]$. If $e$ is a new edge, add $2mn$ to its weight. Here, $n = |U^*| = |V^*|$ and $m = |E^*| = n^2$.
\end{itemize}

The following \Cref{lem:max_to_perfect} establishes the correspondence between the minimum weight perfect matching in $G^*$ and the exact colored matching in $G$:

\begin{lemma}\label{lem:max_to_perfect}
If there is a minimum weight perfect matching $M^*$ satisfying $\phi$ in $G^*$, then $M^* \cap E$ is an exact colored matching $M$ satisfying $\phi$ in $G$.
\end{lemma}
\begin{proof}
    For any exact colored matching $M$ in $G$, the sum of weights $w(M) \leq 2mn$, i.e., smaller or equal to a perfect matching of size $n$ with maximal weight $2m$ for each edge. But the weight of any new edge added for completeness in $G^*$ is $\geq 2mn + 1$. Therefore, any perfect matching containing at least one new adding edge will have a higher sum of weights than the exact colored matching, i.e., it will not have minimal weight. 
\end{proof}

Denote the perfect matching $M^*$ satisfying $\phi$ in $G^*$ as {\em EMC (exact matching with constraint)}. Next, we will prove how to find the minimum weight EMC in $G^*$.
 
\subsubsection{Modified Version of the Isolation Lemma}
~We prove a modified version of the isolation lemma \cite{mulmuley1987matching} to ensure that $G^*$ has a unique minimum weight EMC with probability at least $\frac{1}{2}$. 
    \begin{lemma}\label{lem:isolation}
    \begin{equation}
        \Pr[G^* \text{ has a unique minimum weight EMC}] \geq \frac{1}{2}
    \end{equation}
    \end{lemma}
    \begin{proof}
        The proof is identical to \cite{mulmuley1987matching}. Let us arbitrarily choose an edge $e_i$ from $G^*$. We choose weights for all the edges in $E^*$ randomly except the edge $e_i$. 
    
        Suppose that there are two EMCs in $G^*$: $M_1$ is the minimum weight EMC containing the edge $e_i$ and $M_2$ is the minimum weight EMC not containing the edge $e_i$. Let $W_1$ be the weight of $M_1$ excluding the weight of $x_i$, and $W_2$ be the weight of $M_2$. Define $\alpha_i = M_2 - M_1$. Note the $\alpha_i$ can be either positive or negative. $\alpha_i$ is the threshold for $e_i$ and it does not depend on the weight $w(e_i)$.
        
        If $w(e_i) < \alpha_i$, then weight $W_1 + w(e_i)$, which is the weight of matching $M_1$ containing $e_i$, $< M_2$. Therefore, every minimum weight EMC must contain edge $e_i$.

        If $w(e_i) > \alpha_i$, then weight $W_1 + w(e_i)>M_2$, so $e_i$ is in no minimum weight EMC. 

        If $w(e_i) = \alpha_i$, ambiguity about whether $e_i$ is in an arbitrary minimum weight EMC occurs. Such edge is called {\em singular}. The presence of a singular edge means that a minimum weight EMC is not unique. 

        Since $w(e_i)$ is randomly and uniformly chosen from $\{1, \cdots, 2m\}$:
        \begin{equation}
            P(e_i \text{ is singular}) \leq \frac{1}{2m}
        \end{equation}

        And the probability that there is some singular edge among all $m$ edges is:
        \begin{equation}
            P(\text{there exists a singular edge}) \leq \frac{m}{2m} = \frac{1}{2}
        \end{equation}

        It is equivalent to:
        \begin{equation}
            P(\text{G has a unique minimum weight EMC}) \geq \frac{1}{2}
        \end{equation}
        
    \end{proof}

\subsubsection{Existence of EMC}

We construct a modified adjacency matrix $B$ as follows:
\begin{equation}
\begin{aligned}
B_{u,v} = \begin{cases}
    0 & \text{if } (u,v) \notin E^* \\
    2^{w_e}y_i & \text{if } (u,v) \in E^* \text{ with color } i \\
    2^{w_e} & \text{if } (u,v) \in E^* \text{ is uncolored}
\end{cases}
\end{aligned}
\end{equation}

where $y_1, \cdots, y_k$ are representing the edge colors. $w_e$ is the random weight we assign to each edge $e \in E^*$.

Then we prove the following \Cref{lemma:non_zero_coef}. The proof is identical as \cite{ka2022optimal-AAMAS22}.
    \begin{lemma}\label{lemma:non_zero_coef}
        If there is a EMC in $G^*$, then with probability $\geq \frac{1}{2}$, the coefficient of $\prod_{i=1}^k{y_i}^{\phi_i}$ in $det(B)$ is non-zero.

        Moreover, if there exists a unique minimum weight EMC with weight $w$, then $2^w$ is the highest power of 2 which divides the coefficient of $\prod_{i=1}^k{y_i}^{\phi_i}$.
    \end{lemma}
    
    \begin{proof}
        Since $G^*$ is a complete bipartite graph, $B$ is a $n \times n$ squared matrix. \cut{Now consider $det(B)$. }Let $S_n$ be the set of all permutations of $\{1,\cdots, n\}$. For each permutation $s$, define
        \begin{equation}
            value(s) = \prod_{i=1}^n b_{i,s(i)}
        \end{equation}
          
    where $b_{i,j}$ represents the $(i,j)^{th}$ element of the matrix $B$.

    Notice that each perfect matching corresponds to a permutation in $S_n$. If a permutation doesn't correspond to a perfect matching, then $value(s)=0$. Moreover, for a matching $M$ satisfying the constraint $\phi=(\phi_1, \phi_2,\cdots, \phi_k)$, 
    \begin{equation}
        value(s) = 2^{\sum_{e}w_e}{y_1}^{\phi_1}{y_2}^{\phi_2}\cdots {y_k}^{\phi_k}
    \end{equation}
    
    where $\sum_{e}w_e = w(M)$. 

    Consdier the determinant of the matrix B:
    \begin{equation}
        det(B) = \sum_{s \in S_n}sign(s)value(s) = \sum_{s \in S_n}sign(s)\prod_{i=1}^n b_{i,s(i)}
    \end{equation}

    where $sign(s)$ is $\pm1$ depending on the parity of the permutation $s$.
   
    Moreover, the $det(B)$ can be seen as a polynomial in variables $y_1,y_2, \cdots, y_k$: $det(B) = p(y_1, y_2,\cdots, y_k)$.

     If there is a unique EMC, denote it as $M^*$, then the coefficient of $\prod_{i=1}^k{y_i}^{\phi_i}$ is $2^{w(M^*)}$, which is non-zero. Suppose not, assume that there are EMCs $M_1, M_2, \cdots, M_t$ and the sums of weights of these matchings can be ordered by: $M_1 \leq M_2 \leq \cdots \leq M_t$. Denote the coefficient of ${y_1}^{\phi_1}{y_2}^{\phi_2}$ as $\alpha$:
     \begin{equation}
        \begin{aligned}
        \alpha = &\pm 2^{w(M_1)} \pm 2^{w(M_2)} \pm \cdots \pm 2^{w(M_t)}\\
        = & 2^{w(M_1)}(\pm 1\pm 2^{w(M_2)-w(M_1)} \pm \cdots \pm 2^{w(M_t)-w(M_1)})
        \end{aligned}
     \end{equation}

    By \Cref{lem:isolation}, there is a unique minimum weight EMC with probability at least $\frac{1}{2}$. Note that the term $\pm 2^{w(M_2)-w(M_1)} \pm \cdots \pm 2^{w(M_t)-w(M_1)}$ in the above expression will always be even. Thus if there is a unique minimum weight EMC, $\alpha$ will always be odd and $2^{w(M_1)}$ is the highest power of 2 which divides $\alpha$. If the minimum weight EMC is not unique then the term $\pm 1$ will cancel each other. Therefore, the coefficient is non-zero with probability at least $\frac{1}{2}$.
    
    \end{proof}

By Lemma \ref{lemma:non_zero_coef}, we can output YES if there exists an EMC in $G^*$ with probability at least $\frac{1}{2}$ and output No if there is no such EMC with probability $1$ by checking the coefficient $\alpha$. Next, we prove a modified lemma similar to \cite{mulmuley1987matching} to help us find the minimum weight EMC. 
\subsubsection{Finding the Minimum Weight EMC}
 \begin{lemma}\label{lem: find_edge}
    Let $M^*$ be the unique minimum weight EMC with weight $w$. An edge $(u_i, v_j)$ is in $M^*$ if and only if $\frac{\alpha_{ij}}{2^w}$ is odd, where $\alpha_{ij}$ is the coefficient of $\prod_{i=1}^k{y_i}^{\phi_i}$ in $det(B_{ij})b_{ij}$. $b_{ij}$ is the $(i,j)^{th}$ element in the matrix B, and $B_{ij}$ is the submatrix obtained by removing the $i^{th}$ row and $j^{th}$ column.
\end{lemma}
    
    \begin{proof}
        Note that 
        \begin{equation}
            det(B_{ij})b_{ij} = \sum_{s:s(i)=j}sign(s)value(s)    
        \end{equation}

        $det(B_{ij})b_{ij}$ is a polynomial in variables $y_1,y_2,\cdots, y_k$, and the coefficient of $\prod_{i=1}^k{y_i}^{\phi_i}$ is $\alpha_{ij}$.
        Notice the permutation $s$ with $s(i)=j$ corresponds to the matching containing the edge $(u_i, v_j)$. Therefore, $\alpha_{ij}$ sums up $\pm 2^{w(M)}$ over all perfect matching $M$ both  satisfying the constraint $\phi$ and containing $(u_i, v_j)$.
        
        If $(u_i, v_j) \in M^*$, then the sum $\alpha_{ij}$ will have value $2^{w}$. The remaining permutations have value zero or a higher power of 2. Hence $\frac{\alpha_{ij}}{2^w}$ will be odd. If $(u_i, v_j) \not\in M^*$, all permutations in the sum $\alpha_{ij}$ have value zero or a power of 2 higher than $2^{w}$. Thus $\frac{\alpha_{ij}}{2^w}$ will be even.
    \end{proof}

    By \Cref{lem:isolation,lemma:non_zero_coef}, the \Cref{alg:randomized} correctly finds an exact colored matching $M$ satisfying $\phi$ with probability at least $\frac{1}{2}$ if one exists, and reports "No matching satisfies $\phi$" with probability $1$ otherwise.
    
    Moreover, the only situation in which the algorithm produces incorrect results is when there is an EMC in $G^*$ but the $\alpha$ is zero. The probability of producing incorrect results is at most $\frac{1}{2}$. We can repeat the algorithm from step (2) multiple times to decrease the probability of getting incorrect output.
    
\subsubsection{Time Complexity of Algorithm \ref{alg:randomized}}\label{subsec:randomized_time}
As analyzed in ~\cite{mulmuley1987matching,ka2022optimal-AAMAS22}, the time complexity of \Cref{alg:randomized} is primarily decided by two steps:
    \begin{enumerate}
        \item Computing the determinant $det(B)$ and adjoint matrix $adj(B)$: \citet{mulmuley1987matching} shows that this can be done in $O(\log^2{n})$ parallel time using $O(n^{3.5}m)$ processors by Pan's randomized matrix-inversion algorithm\cite{pan1985fast} for inverting an $n \times n$ matrix whose entries are m-bit integers. Thus this step can be solved in $RNC^2$ time.
        \item Computing the coefficients of $\prod_{i=1}^k{y_i}^{\phi_i}$ in $det(B)$ and $det(B_{ij})b_{ij}$ for each edge $(u_i, v_j)$: \cite{ka2022optimal-AAMAS22} shows that this can be done in $O(n^{k^2})$ time using multi-variate polynomial interpolation through the approach in \cite{hecht2017quadratic}, where $n$ is the size of matrix $B$
    \end{enumerate}
    Therefore, the overall time complexity is $O(n^{k^2}\log^2{n})$, which is polynomial for constant $k$.
    
\cut{
As shown in ~\cite{mulmuley1987matching}, the first step can be solved in $O(\log^2{n})$ time on $O(n^{3.5}m)$ processors by Pan's randomized matrix-inversion algorithm\cite{pan1985fast} for inverting an $n \times n$ matrix whose entries are m-bit integers. Thus this step can be solved in $RNC^2$ time. As shown in \cite{ka2022optimal-AAMAS22}, the second step can be solved by multi-variate polynomial interpolation through the approach in \cite{hecht2017quadratic}. It can be done in $O(n^{k^2})$, where $n$ is the size of matrix $B$. Therefore, the overall time is $O(n^{r^2}\log^2{n})$. Since now we only consider constant $k$ colors, the algorithm runs in polynomial time.
}
    %The first step requires at most $O(n^4)$ time\cite{ka2022optimal-AAMAS22}. As shown in ~\cite{mulmuley1987matching}, it also can be solved in $O(log^2 n)$ time on $O(n^{3.5}m)$ processors by Pan's randomized matrix-inversion algorithm\cite{pan1985fast} for inverting an $n \times n$ matrix whose entries are m-bit integers. Thus this step can be solved in $RNC^2$ time.

    %The second step can be solved by multi-variate polynomial interpolation\cite{ka2022optimal-AAMAS22}. Through the approach in\cite{hecht2017quadratic}, it can be done in time $n^{k^2}$, where $n$ is the size of matrix $B$. Then when $k = O(1)$, i.e. the number of colors on $C$ is constant, this step can be done in polynomial time.
    
    %Thus the overall time is at most $O(n^{r^2+4})$. Since now we only consider constant $k$ colors, the algorithm runs in polynomial time.
